# Supplementary material for: RankingSHAP -- Listwise Feature Attribution Explanations for Ranking Models
Source: arXiv:2403.16085 source file (2025-04-29)
Supplement: Supplementary file 1 [file appendix.tex]

\newpage 

\section{Simulated experiment - additional results. }\label{section:appendix_additional_results}
Here we present additional results for the simulated experiment for some more query scenarios, as well as for the unbiased model from the flowchart in Figure~\ref{figure:model_flow_chart-unbiased}. 

\subsection{Additional query scenarios}\label{section:appendix_additional_query_scenarios}

\input{figures/tex_figures/Toy_example_updated_full}

\subsubsection{Nepotism query}
\header{Description} For this query, one additional candidate from $\text{university}_\text{nepotism}$ with good records for $x_{\text{skill}}$, $x_{\text{exp}}$ and $x_{\text{grade}}$ is considered, but lacking some of the job requirements.

\header{Importance} As we know, the model has picked up on a bias in the data, favoring candidates coming from $\text{university}_\text{nepotism}$, which coincidentally or not is the same university that some people that made past hiring decisions graduated from. 
Hence, for this query we estimate $imp_{\text{rq}}$ to take a smaller value, and $imp_{\text{uni}}$ to take a higher importance value.

\header{Evaluation of the feature attributes}
In Fig.~\ref{figure:synthetic_bar_extended}(b) we see that all approaches correctly pick up on the bias towards  $\text{university}_\text{nepotism}$  by assigning a high value to $x_{\text{uni}}$, while assigning a low value to/ not selecting the usually important $x_{\text{req}}$. 

\subsubsection{International query}

\header{Description}This query considers candidates from universities with different grading schemes. Most candidates meet the job requirements, and none are from $\text{university}_\text{nepotism}$ or $\text{university}_\text{neg-bias}$

\header{Importance}
For this query we estimate $imp_{\text{uni}}$ to take a higher value than for the average query. 
Since candidates from universities with different grading schemes are compared, knowing which university the candidate went to is important for the interpretation of the grades. 

\header{Evaluation of the feature attributes}
By comparing Fig.~\ref{figure:synthetic_bar_extended}(d), with the plot for the average query (a) we see that \method is the only approach assigning $x_{\text{uni}}$  a higher value than for the average query. 

\subsection{Unbiased model explanations}\label{section:appendix_additional_unbiased_model}
\input{figures/tex_figures/Toy-example-bar-unbiased}

\noindent%
The bar chart in Figure~\ref{figure:synthetic_bar_unbiased} shows the feature attribution values from the three considered approaches from Section~\ref{section:experiments_simulated_evaluation} for the same query scenarios as defined in Section~\ref{section:experiments_scenarios}. Comparing the attribution values of different models for different query scenarios like in Figures~\ref{figure:synthetic_bar_extended} and~\ref{figure:synthetic_bar_unbiased} can help us with selecting the least biased model when we have a choice of models of similar performance. 
% \clearpage
% \newpage

\subsection{Additional per candidate analysis}\label{section:appendix_additional_per_query}
Here we provide additional results of the per candidate analysis from Section~\ref{section:toy-example-zoom-in}. 
\input{figures/tex_figures/Toy-example-bar-one_vs_all}
\input{figures/tex_figures/Toy-example-bar-pointwise_shap}
